# Supplementary material for: Phenomenological aspects of supergravity theories in de Sitter vacua
Source: arXiv:1608.08841 source file (2016-08-31)
Supplement: Supplementary file 3 [file myappendix.tex]

\chapter{Appendices}\label{ch:myappendix}

\cleardoublepage
