# Supplementary material for: Phenomenological aspects of supergravity theories in de Sitter vacua
Source: arXiv:1608.08841 source file (2016-08-31)
Supplement: Supplementary file 4 [file appendix_anomalies_old.tex]

\chapter{Anomalies} 

\todo{To Toine: Deze appendix NIET LEZEN. Deze ga ik volledig herschrijven zodat het past in het chiral compensator formulism in deze thesis.}


\section{Some other appendix} \label{Appendix:anomaliesR} 

\red{The action considered is }
\begin{align}\label{yyy}
\mathcal S &= \int d^4x \left\{  d^4\theta {\bf{E}} \left[ (-3/\kappa^2)  S_0^\dagger  e^{2 (\xi/3) V_R} S_0 e^{-\kappa^2 K_0/3}\right],
+ \left[\int d^2 \theta \mathcal E  S_0^3 W(\Phi^i) + \text{h.c.} \right]\right\} \notag \\
\kappa^2 \mathcal K & \equiv  \kappa^2  \mathcal K_0 - 2 \xi V_R.
\end{align}
$\Phi^i$ are matter superfields charged or not under these groups.   $S_0$ is the conformal compensator superfield,
$\bf{E}$ is the superspace measure, $\mathcal E$ is the chiral superspace measure.  $V_R$ is a $U(1)_R$ vector superfield,
$\xi$ is the constant Fayet-Iliopoulos term. In the flat limit $\mathcal S\supset \int d^4\theta \,(\mathcal K_0 - 2 \xi V_R)$. 
If $\mathcal K_0\supset \Phi^\dagger \exp(2 q V_R) \Phi$ then $\mathcal S \supset q \vert \phi \vert^2 -\xi D+D^2/2$ giving $D^2\sim (q\vert\phi\vert^2-\xi)^2$.
The action is invariant under a super-Weyl symmetry (eq.(2.9) in \cite{KL})
 \begin{align}\label{pp}
\lambda \rightarrow e^{-3\tau}\lambda, \quad && {\bf{E}} \rightarrow e^{2\tau +2 \bar \tau} {\bf{E}}, \quad
\qquad \mathcal E\rightarrow e^{6 \tau} \mathcal E, \qquad
\mathcal W_\alpha\rightarrow e^{-3\tau}\,\mathcal W_\alpha, \notag \\
V^{(a)}\rightarrow V^{(a)}, \quad && 
S_0\rightarrow e^{-2 \tau} S_0, \qquad 
\quad W\rightarrow W, \qquad\,\,\,
\bar{\mathcal W}^{\dot\alpha} \rightarrow e^{-3\bar \tau} \bar{\mathcal W}^{\dot\alpha},
\end{align}
with complex parameter $\tau$. Note that the superpotential does not transform, while in our case it does (so super-Weyl transformation is a particular case
of an $R$-symmetry). We thus need an extra $U(1)_R$; under a $U(1)_R$ gauge transformation 
\footnote{This  transformation on $V_R$ corresponds to a gauge transformation
$A_\mu\rightarrow A_\mu+\partial_\mu \rho$ where $\rho=\re\Lambda_{\theta=\bar \theta=0}$. Under this gauge transformation, the scalar  fields transform as:  
$\phi\rightarrow \exp(-i q \rho)\phi$, 
with $D_\mu\phi\equiv (\partial_\mu \phi+ i  g  q A_\mu)\phi$ where $q$ is the charge of  the field $\phi$. 
This is consistent with conventions in the text: $D_\mu \phi^j\equiv \partial_\mu \phi^j-X^j(\phi) A_\mu$, and  $\delta \phi^j=\rho  X^j(\phi)$ 
and the Killing vectors $X^j(\phi)=- i q \phi^j$ for a linearly transformed $\phi$. 
These  conventions are similar to those in \cite{Zwirner} but charges $q$ and $\xi$ of  opposite signs.}
\begin{align} V_R  \rightarrow   V_R + \frac{i}{2} (\Lambda-\Lambda^\dagger),\qquad \bar D\Lambda=0 .  \end{align}
$\mathcal K$ must then transform ($\mathcal K_0$ however is invariatnt)
\begin{align}  \kappa^2 \mathcal K   \rightarrow  \kappa^2 K -  i \xi (\Lambda-\Lambda^\dagger)         .       \end{align}
The action is invariant under $U(1)_R$ if
\begin{align} S_0\rightarrow S_0^\prime = e^{-i\xi/3\Lambda} S_0, \qquad
W\rightarrow W^\prime = e^{+i \xi \Lambda} W\qquad 
\Rightarrow \,\,\,\, R_W=-\xi.
\end{align}
and  $\mathcal G = \kappa^2 \mathcal K+\log \vert W \kappa^{3} \vert^2$ is invariant, too\footnote{
With $W = a e^{b S}$, ($b<0$), under transformation $S\rightarrow S-ic \Lambda$ gives $\xi=-  bc$ and $D^2 \sim (q\vert\phi\vert^2 +bc)^2$.}.
The choice of super-Weyl gauge $S_0=s_0+\theta^2\,F$ can be maintained if we combine the previous  super-Weyl and the $U(1)_R$ transformations such as the conformal compensator remains invariant
(neutral). This is possible provided that \cite{OtherR3}
\begin{align} -2\tau - i (\xi/3) \Lambda=0,\quad \rightarrow \quad \tau=-\frac{i \xi \Lambda}{6}. \end{align}
Thus  $R_\lambda=R_{\mathcal W}=-\xi/2$  according to (\ref{pp}).
We thus work in this gauge which keeps manifest SUSY and holomorphicity  and the compensator is neutral under this $U(1)_R$. 
A consequence is that, according to the transformation of $\bf{E}$,  the gravitino will carry a charge under this new $U(1)_R$.
Further, we also have \begin{align}
 \label{R}
R_{V}=0,\,\,\,\,
R_{\mathcal W}=-\frac{\xi}{2}=R_{\bar D^2 D} \end{align}
With $V\supset \bar \theta \bar \theta \theta\lambda$ then $R_\theta=R_\lambda=-\xi/2$. A superfield of R-charge $Q$ transforms as $\Phi \rightarrow  e^{- i Q \Lambda} \Phi$.
The component form of the action contains, for a superfield $\Phi=(\phi,\psi_\phi)$ \cite{wessbagger}
\begin{align}\mathcal L\supset X^\phi \bar \psi_\phi \bar \lambda + \text{h.c.}\end{align}
$X^\phi$ is the Killing vector of scalar $\phi$ and $\lambda$ the R-gaugino.
For a  superfield with $\Phi\rightarrow e^{- i Q \Lambda} \Phi$  
\begin{align}
 X^\phi \propto i \phi\qquad \Rightarrow \qquad 
R_{\psi_\phi}=R_{\phi} - R_\lambda= Q+\frac{\xi}{2}
\end{align}
which was used in the text. Consider now that $\mathcal K_0$ contains  a dilaton ($S$) dependent term
\begin{align}
\mathcal K_0\supset -\log(S+S^\dagger-\delta  V_R)
\end{align}
which is invariant under our gauged $U(1)_R$ provided
\begin{align}
S\rightarrow S+i \frac{\delta}{2} \Lambda,\quad \delta \text{ real}; \qquad
s\rightarrow s+i  \frac{\delta}{2} \rho,\qquad
\rho\equiv (\re\Lambda) \vert_{\theta=\bar \theta=0}.
\end{align}
For the dilaton $S=(s,\psi_s)$
\begin{align}
X^s=+i\delta, \quad\Rightarrow \quad 
 R_{\psi_s}= -R_\lambda=\frac{\xi}{2}\quad \Rightarrow \quad R_{\phi^s}=R_{\psi_s}+R_\theta=0.
\end{align}
Regarding the gravitino $\psi_{(3/2)}$, from any of the terms of the supergravity Lagrangian 
\begin{align}
L\supset -\frac{1}{2} e D_a \psi_{(3/2)} \sigma \bar \lambda^{a}+ e^{\mathcal K/2} W \bar \psi_{(3/2)}\sigma \bar \psi_{(3/2)}+\text{h.c. } , \end{align}
one obtains the value of $R_{\psi_{3/2}}$ used in the text:
\begin{align}
R_{\psi_{(3/2)}}=R_\lambda=\frac{1}{2} R_W=\frac{-\xi}{2}.
\end{align}


\section{Anomalies with a gauged R-symmetry from a field-theoretic point of view} \label{Appendix:Anomalies-R-Field_Theory}

Consider the Lagrangian in the global SUSY limit, 
\begin{align} \mathcal L =& - \int  d^4\theta \log (S+\bar S -\delta V_R) \notag \\
&+  \frac{1}{16\pi^2 \kappa}  \int  d^2\theta \left[ k_R S \mathcal W_R^\alpha \mathcal W_{R,\alpha} + k_a S \Tr \mathcal W^\alpha_a \mathcal W_{a,\alpha}\right] + \text{ h.c.} ,
\end{align}
where $S$ is the dilaton, \red{$\kappa$ cancels the $\Tr$ factor in non-Abelian case.} 
$k_R$ and $k_a$ are Kac-Moody levels of $U(1)_R$ and of the subgroups $G_a: U(1)_Y$, $SU2)_L$, $SU(3)$  of the Standard Model gauge group. For example for $U(1)_R$, the kinetic terms are given by
\begin{align} \mathcal L \supset \frac{1}{16 g^2} \int d^2\theta k_R S \mathcal W_R^2
\supset k_R \left[ \frac{-1}{4} \re(s) C_{\mu\nu} C^{\mu\nu} +\frac{1}{2} \re(s) D_a^2+ \frac{1}{4}\,\im(s) C_{\mu\nu} \tilde C^{\mu\nu}\right],
\end{align} where \begin{align} \tilde C^{\mu\nu}=1/2\,\epsilon^{\mu\nu\rho\sigma} C_{\rho\sigma} \end{align}. Consider the  shift 
\begin{align} S\rightarrow S+i \frac{\delta}{2} \Lambda(x), \end{align}
and define
\begin{align} C_\alpha=\Tr_{G_\alpha} \left[T(r)^2\,R_\psi \right], \end{align}
where $C_\alpha$ denotes the mixed anomaly $U(1)_R$  with $G_\alpha=U(1)_Y, SU(2)_L$, or  $SU(3)$,  and $R_\psi$ is the $U(1)_R$ charge with fermions transforming as 
\begin{align} \psi\rightarrow e^{-i R_\psi \rho} \psi, \end{align}
with $\rho=\re\Lambda\vert_{\theta= \bar \theta=0}$. Next, $R_\psi$ depend on the Fayet-Iliopoulos  constant ($\xi$) \red{as discussed in previous Appendix}.

The anomalous $U(1)_R$ generates $\Delta  \mathcal L \propto \int d^2\theta [ i C_\alpha \Lambda \mathcal W_a \mathcal W_{a}]$
for each subgroup $G_\alpha$. The shift of the dilaton is the same for all $G_\alpha$ (ignoring $k_\alpha$) then
the ratio $C_\alpha/k_\alpha$ must be identical  for all $G_\alpha$ for anomalies to cancel. Also taking the $U(1)^3_R$ and $U(1)_R$-gravitational anomaly, then one has the result
\begin{align}
- 4 \pi^2 \delta = \frac{2 C_\alpha}{k_\alpha} = \frac{(2/3)  \Tr R_\psi^3}{k_R}=\frac{1}{12} \Tr \,R_\psi, \label{an1}
\end{align}
In the paper we kept $k_R=1$. The gauge couplings constants are  then  \begin{align} k_\alpha \langle \text{Re}(s) \rangle \equiv 1/g_\alpha^2 \end{align}.

Regarding the mixed gravitational anomaly (last term above) this is seen from the action 
\begin{align} \mathcal L  \supset  \frac{-1}{4} \text{Im} (s) \mathcal R \tilde{\mathcal R} \qquad
\Delta \mathcal L_{\text{axion}}= -\frac{\rho}{8} \delta \mathcal R \tilde{\mathcal R}, \qquad
\Delta \mathcal L_{\text{anomaly}}= \frac{\rho}{384 \pi^2} \Tr [R_\psi] \mathcal R \tilde{\mathcal R} \notag
\end{align}
and use $\Delta L_{\text{axion}}+\Delta L_{\text{anomaly}}=0$. However, unlike in heterotic string, in supergravity,  
  $\mathcal R \tilde{\mathcal R}$ term can have a different coefficient from $\Im(s)$ since it is not part of the leading order action.

In the text we used the notation $W=a e^{b S}$, with $b<0$ and  $S \rightarrow S-i c \Lambda$ giving $\delta/2=-c$. The anomaly condition (\ref{an1}) becomes
\begin{align} 4\pi^2 c = \frac{C_\alpha}{k_\alpha}=\frac{(1/3) \Tr R_\psi^3}{k_R}=\frac{1}{24} \Tr[R_\psi]. \label{an2} \end{align}
This result was compared against the more general supergravity results in Section~\ref{sec:Anomalies-FI}.


\cleardoublepage
